# Supplementary material for: Intrinsic Photon Loss at the Interface of Superconducting Devices
Source: arXiv:1909.04720 ancillary file (2020-10-02)
Supplement: Supplementary file 1 [file SupplementalIntrinsicEnergyLossInterface.pdf]

# Supplemental Material for “Intrinsic photon loss at the interface of superconducting devices”

Igor Diniz<sup>1,2,\*</sup> and Rogério de Sousa<sup>1</sup>

<sup>1</sup>*Department of Physics and Astronomy, University of Victoria,  
Victoria, British Columbia, Canada V8W 2Y2*

<sup>2</sup>*Instituto de Ciências Exatas, Universidade Federal Rural do Rio de Janeiro, Seropédica, Brazil*  
(Dated: March 9, 2020)

Section I provides a summary of the impact of piezoelectricity on acoustic phonons, and the assumptions made to reach the simplified model with one phonon branch. Section II describes our estimates for the piezoelectric vector in bulk piezoelectric materials,  $\mathbf{g}_B$ . Section III describes how the piezoelectric vector  $\mathbf{g}_I$  for the sapphire/vacuum interface can be extracted from recent first-principles calculations. Sections IV and V describes our theory for estimating the piezoelectric vector  $\mathbf{g}_I$  for the metal/vacuum and dielectric/metal interfaces, respectively. Finally, Section VI provides tables with all material parameters used to compute the values for the predicted piezoelectric constants and loss tangents in Table I and II of the main paper.

---

\* igordiniz@ufrj.br

## I. IMPACT OF PIEZOELECTRICITY ON ACOUSTIC PHONONS

The basic equations describing the piezoelectric effect are given by [1]

$$D_i = \sum_j \epsilon_{ij} E_j + \sum_{j,k} e_{i,jk} \varepsilon_{jk} \quad (1a)$$

$$\sigma_{jk} = - \sum_i e_{i,jk} E_i + \sum_{l,m} C_{jk,lm} \varepsilon_{lm}. \quad (1b)$$

Here the subscripts  $i, j, k, l, m = x, y, z$  label cartesian components of vectors and tensors. The electric displacement vector is equal to  $\mathbf{D} = \epsilon_0 \mathbf{E} + \mathbf{P}$ , where  $\epsilon_0$  is the dielectric constant for the vacuum,  $\mathbf{E}$  is the external electric field, and  $\mathbf{P}$  is the material's electric polarization (dimensions of charge over area, C/m<sup>2</sup>). The dielectric tensor  $\epsilon_{ij}$  is related to the dimensionless electric susceptibility  $\chi_{ij}$ ,

$$\epsilon_{ij} = \epsilon_0 (\delta_{ij} + \chi_{ij}), \quad (2)$$

and should not be confused with the strain tensor,

$$\varepsilon_{ij} = \frac{1}{2} \left( \frac{\partial u_i}{\partial x_j} + \frac{\partial u_j}{\partial x_i} \right), \quad (3)$$

where  $\mathbf{u}(\mathbf{r})$  is the atomic displacement vector (displacement of material's atoms with respect to their equilibrium positions in the crystal). Note that  $\varepsilon_{ij}$  is dimensionless. The other quantities are the stress tensor  $\sigma_{ij}$  and elastic constants  $C_{ij,kl}$ , both with dimensions of pressure. Finally,  $e_{i,jk}$  are the coefficients of the piezoelectric tensor with dimensions of polarization (C/m<sup>2</sup>). The way it appears in Eq. (1) is dictated by the thermodynamic relations:

$$e_{i,jk} = \left( \frac{\partial D_i}{\partial \varepsilon_{jk}} \right)_{\mathbf{E}, T} = - \left( \frac{\partial \sigma_{jk}}{\partial E_i} \right)_{\boldsymbol{\varepsilon}, T} = - \frac{1}{V} \left( \frac{\partial^2 F}{\partial E_i \partial \varepsilon_{jk}} \right)_T, \quad (4)$$

where  $F(T, \mathbf{E}, \boldsymbol{\varepsilon}) = U - TS$  is the free energy of the material.

The atomic displacement vector for acoustic phonons is given by

$$\mathbf{u}(\mathbf{r}) = \sum_{\mathbf{k}, \lambda} \hat{\boldsymbol{\eta}}_{\mathbf{k}, \lambda} \sqrt{\frac{\hbar}{2\rho V \omega_{\mathbf{k}, \lambda}}} \left( b_{\mathbf{k}, \lambda} e^{i\mathbf{k} \cdot \mathbf{r}} + b_{\mathbf{k}, \lambda}^\dagger e^{-i\mathbf{k} \cdot \mathbf{r}} \right), \quad (5)$$

where  $b_{\mathbf{k}, \lambda}^\dagger$  and  $b_{\mathbf{k}, \lambda}$  are creation and destruction operators for a phonon with wavevector  $\mathbf{k}$  and polarization mode  $\lambda = 1, 2, 3$ . For each  $\mathbf{k}$ , the three unit vectors  $\hat{\boldsymbol{\eta}}_{\mathbf{k}, \lambda}$  are mutually orthogonal; they describe the phonon's polarization direction. The phonon frequencies  $\omega_{\mathbf{k}, \lambda}$  can be approximated by  $v|\mathbf{k}|$  for a suitable phonon velocity  $v$  when  $k$  is much smaller than  $1/a$ , the material's lattice constant. Finally,  $\rho$  and  $V$  are the material's mass density and volume. From Eqs. (1a), (3), and (5) we derive an explicit expression for the acoustic phonon *electric polarization*:

$$\begin{aligned} P_i &= \sum_{l, m} e_{i, lm} \varepsilon_{lm} \\ &= \sum_{\mathbf{k}, \lambda} \sqrt{\frac{\hbar k^2}{2\rho V \omega_{\mathbf{k}, \lambda}}} \left\{ \sum_{l, m} \frac{e_{i, lm}}{2} \left[ (\hat{e}_l \cdot \hat{\boldsymbol{\eta}}_{\mathbf{k}, \lambda}) (\hat{\mathbf{k}} \cdot \hat{e}_m) + (\hat{e}_m \cdot \hat{\boldsymbol{\eta}}_{\mathbf{k}, \lambda}) (\hat{\mathbf{k}} \cdot \hat{e}_l) \right] \right\} i \left( b_{\mathbf{k}, \lambda} e^{i\mathbf{k} \cdot \mathbf{r}} - b_{\mathbf{k}, \lambda}^\dagger e^{-i\mathbf{k} \cdot \mathbf{r}} \right). \end{aligned} \quad (6)$$

This expression is quite difficult to evaluate for actual piezoelectric materials, whose phonon polarization directions  $\hat{\boldsymbol{\eta}}_{\mathbf{k}, \lambda}$  are only purely longitudinal ( $\hat{\boldsymbol{\eta}}_{\mathbf{k}, \lambda=L} = \hat{\mathbf{k}}$ ) or transverse ( $\hat{\boldsymbol{\eta}}_{\mathbf{k}, \lambda=T1, T2} \perp \hat{\mathbf{k}}$ ) when  $\mathbf{k}$  lies along a high symmetry direction in the material. Similarly, the phonon velocities (and frequencies) are highly dependent on the branch  $\lambda$  and the propagation direction  $\mathbf{k}$ .

In many cases, such as when calculating energy loss in bulk materials, it makes sense to average over all phonon propagation directions  $\hat{\mathbf{k}}$ . As we now show, this reduces Eq. (6) to a much simpler expression that involves only a single “effective phonon branch”. When we go through a Fermi's golden rule calculation of phonon emission/absorption, the matrix elements involving different phonon operators  $b_{\mathbf{k}, \lambda}^\dagger$  and  $b_{\mathbf{k}', \lambda'}$  are necessarily equal to zero unless  $\mathbf{k} = \mathbf{k}'$  and  $\lambda = \lambda'$ . Fermi's golden rule becomes proportional to

$$g_i^2 = \sum_{\lambda=1,2,3} \left\langle \left\{ \sum_{l, m} \frac{e_{i, lm}}{2} \left[ (\hat{e}_l \cdot \hat{\boldsymbol{\eta}}_{\mathbf{k}, \lambda}) (\hat{\mathbf{k}} \cdot \hat{e}_m) + (\hat{e}_m \cdot \hat{\boldsymbol{\eta}}_{\mathbf{k}, \lambda}) (\hat{\mathbf{k}} \cdot \hat{e}_l) \right] \right\}^2 \right\rangle_{\hat{\mathbf{k}}}, \quad (7)$$

where  $\langle \cdot \rangle_{\mathbf{k}}$  denotes an average over all phonon propagation directions.

The values of  $g_i$  obtained from Eq. (7) turn out to be independent of the phonon polarization directions  $\hat{\mathbf{n}}_{\mathbf{k},\lambda}$ , leading to the following general result:

$$g_i^2 = \frac{1}{3} \sum_{l,m} e_{i,lm}^2 = \frac{1}{3} \sum_{I=1}^3 e_{i,I}^2 + \frac{2}{3} \sum_{I=4}^6 e_{i,I}^2, \quad (8)$$

the last expression in the Voigt notation (pairs of cartesian indexes denoted by a single number,  $I \leftrightarrow ij$ , with  $1 \leftrightarrow xx, 2 \leftrightarrow yy, 3 \leftrightarrow zz, 4 \leftrightarrow yz, 5 \leftrightarrow xz, 6 \leftrightarrow xy$ ).

The vector  $\mathbf{g}$  is denoted “piezoelectric vector”. With this definition the phonon’s electric polarization is approximated by

$$P_i = g_i \sum_{\mathbf{k}} \sqrt{\frac{\hbar \omega_{\mathbf{k}}}{2 \rho V v^2}} i \left( b_{\mathbf{k}} e^{i\mathbf{k} \cdot \mathbf{r}} - b_{\mathbf{k}}^\dagger e^{-i\mathbf{k} \cdot \mathbf{r}} \right), \quad (9)$$

which is Eq. (3) in the main paper. Here  $b_{\mathbf{k}}^\dagger$  creates an effective phonon with frequency  $\omega_{\mathbf{k}} = v|\mathbf{k}|$ , where  $v$  is an average phonon velocity for the material. Note that this expression is equivalent to the well known  $\mathbf{P} = \mathbf{g} \nabla \cdot \mathbf{u}$  approximation frequently employed in the literature. The latter depends on a single phonon provided that the branches are purely longitudinal/transverse.

## II. PIEZOELECTRIC VECTOR FOR BULK MATERIALS

The piezoelectric constants  $e_{i,jk}$  are fully characterized for bulk crystalline SiO<sub>2</sub> ( $\alpha$ -Quartz). Only five out of the eighteen  $e_{i,jk}$  are non-zero:  $e_{x,1} = -e_{x,2} = -e_{y,6} \equiv e_{11}$  and  $e_{x,4} = -e_{y,5} \equiv e_{14}$ . Measurements at  $T = 5$  K yield  $e_{11} = 0.07$  C/m<sup>2</sup> and  $e_{14} = -0.03$  C/m<sup>2</sup> [2]. From Eq. (8) we get  $g_x = g_y = 0.06$  C/m<sup>2</sup>, and  $g_z = 0$ . Therefore,

$$\mathbf{g}_B^{\alpha\text{-Quartz}} = 0.09 \frac{1}{\sqrt{2}} (1, 1, 0) \frac{\text{C}}{\text{m}^2}. \quad (10)$$

We are not aware of measurements of piezoelectric coefficients for Nb<sub>2</sub>O<sub>5</sub>. Consider other transition metal oxides: LiNbO<sub>3</sub> has  $|e_{i,jk}| = 0.2 - 1.3$  C/m<sup>2</sup>, and ZnO has  $|e_{i,jk}| = 0.6 - 1.3$  C/m<sup>2</sup> [3]. PbTiO<sub>3</sub> has  $|e_{i,jk}| = 1 - 4$  C/m<sup>2</sup> [4]. Based on these typical values observed for transition metal oxides, we estimate  $|\mathbf{g}_B| \sim 1$  C/m<sup>2</sup> for Nb<sub>2</sub>O<sub>5</sub>.

## III. PIEZOELECTRIC VECTOR FOR THE SAPPHIRE/VACUUM INTERFACE

The piezoelectric tensor coefficients were calculated for the sapphire/vacuum interface using first principles calculations [5] ( $\hat{z}$  was perpendicular to the aluminum terminated surface, denoted  $\alpha\text{-Al}_2\text{O}_3(0001)$  in the Bravais-Miller system). The calculation is particularly interesting because sapphire is not piezoelectric in the bulk; however its surface develops a spontaneous electric dipole moment. In [5] the surface dipole is shown to change under strain, leading to piezoelectricity. Their most sophisticated calculation led to  $e_{z,xx} = e_{z,yy} = -0.16$  C/m<sup>2</sup> (See end of Section III-A in [5]). The value of  $e_{z,zz}$  was not calculated, but it is safe to assume it is approximately equal to  $e_{z,xx}$ . The other “shear” coefficients  $e_{z,yz}, e_{z,xz}, e_{z,xy}$  are expected to be much smaller so we approximate them by zero (note that  $e_{i,jk} = 0$  for  $i = x, y$  because by symmetry the surface dipole is along  $\hat{z}$ ). Using Eq. (8) we get

$$\mathbf{g}_I^{\text{sapphire/vacuum}} = 0.16 (0, 0, 1) t_I \delta(z) \frac{\text{C}}{\text{m}^2}, \quad (11)$$

with the surface assumed to be located at  $z = 0$ . Moreover, as discussed in [5] it makes sense to associate the thickness of the surface dipole layer to be the height of one bulk structural unit in the  $z$  direction,  $t_I = c/6 = 2.17$  Å.

## IV. PIEZOELECTRIC VECTOR FOR THE METAL/VACUUM INTERFACE

When an electric field is applied to a metal, an areal charge density equal to  $\epsilon_0 \mathbf{E} \cdot \hat{\mathbf{n}}$  is induced at each surface ( $\hat{\mathbf{n}}$  is the unit vector normal to the surface). This charge density screens out the electric field inside the metal. The induced charge density has an average thickness of less than 2 Å (See Fig. I.5 of [6]), so we can assume it is concentrated

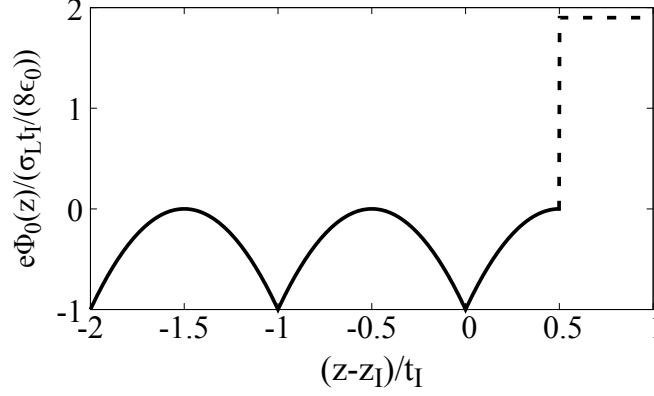

FIG. 1. Confining potential for electrons in the jellium model for a metal/vacuum interface. The solid line is obtained from Eq. (15), and the dashed line is the work function potential.

within the two topmost atomic layers, i.e., within  $t_I$  (which equals the distance between the atomic layer forming the interface and the one immediately below it). The induced charge density affects electrostatic forces leading to non-zero strain within these two atomic layers. The change in electrostatic energy linear in  $\mathbf{E}$  is exactly equal to

$$\frac{\delta U_{\text{elec}}}{V} = \delta \rho_e(\mathbf{r}) \Phi_0(\mathbf{r}), \quad (12)$$

where  $\delta \rho_e(\mathbf{r}) = \epsilon_0 E_z \delta(z - z_I)$  is the induced charge density, and  $\Phi_0(\mathbf{r})$  is the electrostatic potential at  $\mathbf{E} = \mathbf{0}$  (for simplicity we assume  $\hat{\mathbf{n}} = \hat{\mathbf{z}}$  and the layer of cations forming the interface is located at  $z_I$ ). Under the assumption that Eq. (12) dominates the part of the free energy that is linear in  $\mathbf{E}$ , Eq. (4) leads to the following expression for the piezoelectric coefficients:

$$e_{z,jk} = -\frac{1}{V} \frac{\partial^2 U_{\text{elec}}}{\partial E_z \partial \varepsilon_{jk}} = -\epsilon_0 \delta(z - z_I) \left. \frac{\partial \Phi_0(\mathbf{r})}{\partial \varepsilon_{jk}} \right|_{\varepsilon_{jk}=0}. \quad (13)$$

We calculate  $\Phi_0(\mathbf{r})$  assuming the *jellium* model for the metal: A lattice of atomic cations with charge  $Q$  surrounded by a homogeneous electron charge density. Each atomic layer of  $N_I$  cations is made electrically neutral by a constant electron charge density of  $-N_I Q / (A t_I)$ , extending  $t_I/2$  above/below the cation layer. Use Gauss' law for a box with surface parallel to the interface at  $z_{\text{top}} = z$  and at  $z_{\text{bottom}} = z_I - (n + 1/2)t_I$  for some integer  $n$  so that  $z_{\text{bottom}} < z_{\text{top}}$ . The field at  $z_{\text{bottom}}$  is zero, hence the field at  $z$  becomes

$$E_z(z) = \frac{\sigma_I}{\epsilon_0} \left\{ - \left[ \left( \frac{z - z_I}{t_I} \right) - \text{int} \left( \frac{z - z_I}{t_I} \right) \right] + \frac{1}{2} \text{sign} \left( \frac{z - z_I}{t_I} \right) \right\}, \quad (14)$$

where  $\sigma_I = N_I Q / A$  is the charge density associated to the layer of cations. The functions  $\text{int}(x)$  and  $\text{sign}(x)$  output the integer part of  $x$  and the sign of  $x$  (with  $\text{sign}(0) = +1$ ), respectively. The electric potential is obtained from  $\Phi_0(z) = -\int_{\infty}^z E_z(z') dz'$  leading to

$$\Phi_0(z) = \frac{\sigma_I t_I}{2\epsilon_0} \left\{ \left( \frac{z - z_I}{t_I} \right) - \text{int} \left( \frac{z - z_I}{t_I} \right) - \frac{1}{2} \text{sign} \left( \frac{z - z_I}{t_I} \right) \right\}^2. \quad (15)$$

The resulting confining potential for electrons  $e\Phi_0(z)$  is plotted in Fig. 1 ( $e < 0$  is the electron charge), where we also included the energy barrier confining electrons to the surface (work function potential). The latter is assumed to be independent of strain.

We can now evaluate the piezoelectric coefficients using Eq. (13). The impact of strain is to change  $t_I \rightarrow t_I(1 + \varepsilon_{zz})$ , and  $A \rightarrow A(1 + \varepsilon_{xx})(1 + \varepsilon_{yy})$ , leading to

$$e_{z,xx} = e_{z,yy} = \frac{\sigma_I}{8} t_I \delta(z - z_I), \quad (16a)$$

$$e_{z,zz} = -\frac{\sigma_I}{8} t_I \delta(z - z_I), \quad (16b)$$

and all other coefficients equal to zero. Here  $\sigma_I = N_I Q/A$  is the charge density for the cations forming the interface layer (the topmost layer of ions). Using Eq. (8) we get the piezoelectric vector for the metal/vacuum interface. With  $\hat{z} = (0, 0, 1)$  pointing perpendicular to the interface at  $z_I = 0$ ,

$$\mathbf{g}_I^{\text{metal/vacuum}} = \frac{\sigma_I}{8}(0, 0, 1)t_I\delta(z). \quad (17)$$

## V. PIEZOELECTRIC VECTOR FOR THE DIELECTRIC/METAL INTERFACE

Consider an infinite metal/dielectric interface perpendicular to  $\hat{z}$  with metal in the upper half ( $z > 0$ ) and dielectric in the lower half ( $z < 0$ ). At  $\mathbf{E} = \mathbf{0}$  the electrons in the metal will form an image surface dipole layer in order to cancel out the spontaneous surface electric dipole appearing in the dielectric side. As a result we expect the piezoelectric coefficients on the dielectric side to be greatly reduced in comparison to the dielectric/vacuum configuration. However, a similar mechanism to the one described in Section IV above will still be present, and we believe it will give the dominant contribution to  $e_{i,jk}$  in the dielectric/metal case.

The difference from Section IV is the presence of two screening charge densities under the application of  $\mathbf{E}$ . On the dielectric side we get the usual screening polarization,  $\sigma_{\text{dielec}} = \chi_{zz}/(1 + \chi_{zz})\epsilon_0 E_z$ , and on the metal side we get  $\sigma_{\text{metal}} = -\epsilon_0 E_z$  (the minus sign because  $\mathbf{E} \parallel -\hat{n}$  for the metal). Adding both contributions we get

$$\delta\rho_e(\mathbf{r}) = -\frac{\epsilon_0^2 E_z}{\epsilon_{zz}}\delta(z - z_I). \quad (18)$$

Without any further information about the charge distribution at the interface we assume the electric potential on the metal side can be approximated by Eq. (15). This leads to

$$e_{z,xx} = e_{z,yy} = -\frac{\sigma_I \epsilon_0}{8\epsilon_{zz}}t_I\delta(z - z_I), \quad (19a)$$

$$e_{z,zz} = \frac{\sigma_I \epsilon_0}{8\epsilon_{zz}}t_I\delta(z - z_I), \quad (19b)$$

where  $\sigma_I = N_I Q/A$  is the charge density for the interface cation layer on the metal side. Using Eq. (8) we get the piezoelectric vector for the dielectric/metal interface:

$$\mathbf{g}_I^{\text{dielectric/metal}} = \frac{\sigma_I \epsilon_0}{8\epsilon_{zz}}(0, 0, 1)t_I\delta(z). \quad (20)$$

This is a factor of  $\epsilon_0/\epsilon_{zz}$  smaller than the metal/vacuum interface, showing that the dielectric acts as a “buffer” for the interface piezoelectric effect in the metal.

## VI. TABLE OF MATERIAL PARAMETERS

TABLE I. Material parameters used for computing the piezoelectric vectors  $\mathbf{g}$  and the loss tangent. Note that for a metal/dielectric interface the value of  $\epsilon$  in Eq. (8) of the main paper is the dielectric constant of the insulator only (where most of the photon’s  $\psi(\mathbf{r})$  is located).

|                                | $Q/ e $ | $\sigma_I$ (C/m <sup>2</sup> ) | $\epsilon/\epsilon_0$ | $\rho$ (g/cm <sup>3</sup> ) | $v$ (km/s) | Reference |
|--------------------------------|---------|--------------------------------|-----------------------|-----------------------------|------------|-----------|
| Al                             | 3       | 5.86                           | 1                     | 2.70                        | 6.51       | [7]       |
| Nb                             | 1       | 1.47                           | 1                     | 8.57                        | 5.43       | [8]       |
| Al <sub>2</sub> O <sub>3</sub> |         |                                | 11.59                 | 3.97                        | 11.2       | [9]       |
| SiO <sub>2</sub>               |         |                                | 4.64                  | 2.66                        | 6.40       | [9]       |
| Nb <sub>2</sub> O <sub>5</sub> |         |                                | 33                    | 4.60                        | 5.43       | [10]      |

[1] D. W. Snoke, *Solid State Physics: Essential Concepts*, 2nd ed. (Cambridge University Press, U.K., 2020).

- [2] R. Tarumi, K. Nakamura, H. Ogi, and M. Hirao, *J. Appl. Phys.* **102**, 113508 (2007).
- [3] M. A. Fraga, H. Furlan, R. Pessoa, and M. Massi, *Microsyst. Technol.* **20**, 9 (2014).
- [4] Z. Li, M. Grimsditch, X. Xu, and S. K. Chan, *Ferroelectrics* **141**, 313 (1993).
- [5] A. B. Georgescu and S. Ismail-Beigi, *Phys. Rev. Appl.* **11**, 064065 (2019).
- [6] J. D. Jackson, *Classical Electrodynamics*, 3rd ed. (Wiley, New York, 1998).
- [7] G. N. Kamm and G. A. Alers, *J. Appl. Phys.* **35**, 327 (1964).
- [8] W. C. Rubell and F. R. Brotzen, *J. Appl. Phys.* **43**, 3306 (1972).
- [9] H. Y. Hao and H. J. Maris, *Phys. Rev. B* **63**, 224301 (2001).
- [10] A. Romanenko and D. I. Schuster, *Phys. Rev. Lett.* **119**, 264801 (2017).
